# Supplementary material for: Learning Fair Scoring Functions: Bipartite Ranking under ROC-based Fairness Constraints
Source: arXiv:2002.08159 source file (2021-02-25)
Supplement: Supplementary file 2 [file table.tex]

\begin{tabular}{cccccccc} 
\toprule 
$\lambda / \lambda_H$ & $\lambda_\text{reg}$ & $\auc$ & $\Delta \auc$ 
& $|\Delta_H(\frac{1}{8})|$ & $|\Delta_H(\frac{3}{4})|$ & $L_\lambda$ & $L_\Lambda$ \\ 
\midrule 
$0.00$ & $0.050$ & $0.90$ & $0.04$ & $0.33$ & $0.37$ & $0.90$ & $0.90$ \\ 
$0.25$ & $0.050$ & $0.87$ & $0.04$ & $0.06$ & $0.00$ & $0.86$ & $0.85$ \\ 
$0.50$ & $1.000$ & $0.86$ & $0.04$ & $0.02$ & $0.00$ & $0.84$ & $0.85$ \\ 
$1.00$ & $1.000$ & $0.86$ & $0.05$ & $0.02$ & $0.01$ & $0.81$ & $0.83$ \\ 
$5.00$ & $1.000$ & $0.86$ & $0.05$ & $0.02$ & $0.00$ & $0.64$ & $0.74$ \\ 
$10.00$ & $1.000$ & $0.85$ & $0.04$ & $0.01$ & $0.06$ & $0.40$ & $0.12$ \\ 
\bottomrule 
\end{tabular}
