# Supplementary material for: Learning Fair Scoring Functions: Bipartite Ranking under ROC-based Fairness Constraints
Source: arXiv:2002.08159 source file (2021-02-25)
Supplement: Supplementary file 3 [file table.tex]

\begin{tabular}{cccccccc} 
\toprule 
$\lambda / \lambda_H$ & $\lambda_\text{reg}$ & $\auc$ & $\Delta \auc$ 
& $|\Delta_H(\frac{1}{8})|$ & $|\Delta_H(\frac{3}{4})|$ & $L_\lambda$ & $L_\Lambda$ \\ 
\midrule 
$0.00$ & $0.050$ & $0.94$ & $0.13$ & $0.10$ & $0.20$ & $0.94$ & $0.94$ \\ 
$0.25$ & $0.100$ & $0.94$ & $0.12$ & $0.09$ & $0.18$ & $0.91$ & $0.87$ \\ 
$0.50$ & $0.100$ & $0.93$ & $0.11$ & $0.10$ & $0.19$ & $0.87$ & $0.78$ \\ 
$1.00$ & $0.500$ & $0.88$ & $0.08$ & $0.12$ & $0.23$ & $0.79$ & $0.53$ \\ 
$5.00$ & $0.500$ & $0.81$ & $0.03$ & $0.12$ & $0.24$ & $0.65$ & $-0.98$ \\ 
$10.00$ & $0.010$ & $0.77$ & $0.02$ & $0.12$ & $0.20$ & $0.54$ & $-2.41$ \\ 
\bottomrule 
\end{tabular}
