# Supplementary material for: Learning Fair Scoring Functions: Bipartite Ranking under ROC-based Fairness Constraints
Source: arXiv:2002.08159 source file (2021-02-25)
Supplement: Supplementary file 5 [file table.tex]

\begin{tabular}{cccccccc} 
\toprule 
$\lambda / \lambda_H$ & $\lambda_\text{reg}$ & $\auc$ & $\Delta \auc$ 
& $|\Delta_H(\frac{1}{8})|$ & $|\Delta_H(\frac{3}{4})|$ & $L_\lambda$ & $L_\Lambda$ \\ 
\midrule 
$0.00$ & $0.050$ & $0.72$ & $0.21$ & $0.26$ & $0.37$ & $0.72$ & $0.72$ \\ 
$0.25$ & $0.050$ & $0.72$ & $0.02$ & $0.08$ & $0.07$ & $0.71$ & $0.68$ \\ 
$0.50$ & $0.050$ & $0.72$ & $0.01$ & $0.05$ & $0.05$ & $0.71$ & $0.67$ \\ 
$1.00$ & $0.100$ & $0.72$ & $0.05$ & $0.09$ & $0.09$ & $0.67$ & $0.54$ \\ 
$5.00$ & $0.005$ & $0.71$ & $0.07$ & $0.07$ & $0.12$ & $0.39$ & $-0.26$ \\ 
$10.00$ & $0.010$ & $0.71$ & $0.02$ & $0.05$ & $0.08$ & $0.48$ & $-0.56$ \\ 
\bottomrule 
\end{tabular}
