# Supplementary material for: Learning Fair Scoring Functions: Bipartite Ranking under ROC-based Fairness Constraints
Source: arXiv:2002.08159 source file (2021-02-25)
Supplement: Supplementary file 7 [file table.tex]

\begin{tabular}{cccccccc} 
\toprule 
$\lambda / \lambda_H$ & $\lambda_\text{reg}$ & $\auc$ & $\Delta \auc$ 
& $|\Delta_H(\frac{1}{8})|$ & $|\Delta_H(\frac{3}{4})|$ & $L_\lambda$ & $L_\Lambda$ \\ 
\midrule 
$0.00$ & $0.500$ & $0.75$ & $0.07$ & $0.01$ & $0.26$ & $0.75$ & $0.75$ \\ 
$0.25$ & $0.500$ & $0.77$ & $0.06$ & $0.02$ & $0.05$ & $0.75$ & $0.75$ \\ 
$0.50$ & $0.500$ & $0.77$ & $0.05$ & $0.06$ & $0.09$ & $0.74$ & $0.69$ \\ 
$1.00$ & $0.500$ & $0.78$ & $0.05$ & $0.00$ & $0.02$ & $0.73$ & $0.75$ \\ 
$5.00$ & $0.500$ & $0.77$ & $0.04$ & $0.02$ & $0.03$ & $0.59$ & $0.51$ \\ 
$10.00$ & $0.500$ & $0.76$ & $0.05$ & $0.02$ & $0.08$ & $0.24$ & $-0.25$ \\ 
\bottomrule 
\end{tabular}
