# Supplementary material for: Learning Fair Scoring Functions: Bipartite Ranking under ROC-based Fairness Constraints
Source: arXiv:2002.08159 source file (2021-02-25)
Supplement: Supplementary file 9 [file 9-appendix-expes-illustrations.tex]

% \section{Experimental details - illustrations}
% \subsection{Run dynamics}
% 
% \robin{list of figures}
% 
% \begin{figure}[h]
%     \centering
%     \subfigure{
%     \includegraphics[width=0.25\linewidth]{figures/expes/toy1/dyn/med_lambda/cost.pdf}
%     \includegraphics[width=0.25\linewidth]{figures/expes/toy1/dyn/med_lambda/auc.pdf}
%     \includegraphics[width=0.25\linewidth]{figures/expes/toy1/dyn/med_lambda/f_auc.pdf}
%     }
%     \subfigure[$\lambda=0.1$]{
%     \includegraphics[width=0.25\linewidth]{figures/expes/toy1/dyn/med_lambda/c.pdf}
%     \includegraphics[width=0.25\linewidth]{figures/expes/toy1/dyn/med_lambda/l2.pdf}
%     }
%     \subfigure[a]{
%     \includegraphics[width=0.25\linewidth]{figures/expes/toy1/dyn/high_lambda/cost.pdf}
%     \includegraphics[width=0.25\linewidth]{figures/expes/toy1/dyn/high_lambda/auc.pdf}
%     \includegraphics[width=0.25\linewidth]{figures/expes/toy1/dyn/high_lambda/f_auc.pdf}
%     }
%     \subfigure[$\lambda = 1$]{
%     \includegraphics[width=0.25\linewidth]{figures/expes/toy1/dyn/high_lambda/c.pdf}
%     \includegraphics[width=0.25\linewidth]{figures/expes/toy1/dyn/high_lambda/l2.pdf}
%     }
%     \caption{Dynamics runs of \cref{alg:sec3} on \cref{example-square}.
%     % Note that, in the case of $\lambda=0.1$, since the constraint has little effect
%     % on the solution, the parameter $c$ drifts all the way to $1$.
%     }\label{fig:dynamics_toy1}
% \end{figure}
% 
% \begin{figure}[h]
%     \centering
%     \subfigure{
%     \includegraphics[width=0.25\linewidth]{figures/expes/toy2/dyn_auc/med_lambda/cost.pdf}
%     \includegraphics[width=0.25\linewidth]{figures/expes/toy2/dyn_auc/med_lambda/auc.pdf}
%     \includegraphics[width=0.25\linewidth]{figures/expes/toy2/dyn_auc/med_lambda/f_auc.pdf}
%     }
%     \subfigure[$\lambda=0.1$]{
%     \includegraphics[width=0.25\linewidth]{figures/expes/toy2/dyn_auc/med_lambda/c.pdf}
%     \includegraphics[width=0.25\linewidth]{figures/expes/toy2/dyn_auc/med_lambda/l2.pdf}
%     }
%     \subfigure{
%     \includegraphics[width=0.25\linewidth]{figures/expes/toy2/dyn_auc/high_lambda/cost.pdf}
%     \includegraphics[width=0.25\linewidth]{figures/expes/toy2/dyn_auc/high_lambda/auc.pdf}
%     \includegraphics[width=0.25\linewidth]{figures/expes/toy2/dyn_auc/high_lambda/f_auc.pdf}
%     }
%     \subfigure[$\lambda = 1$]{
%     \includegraphics[width=0.25\linewidth]{figures/expes/toy2/dyn_auc/high_lambda/c.pdf}
%     \includegraphics[width=0.25\linewidth]{figures/expes/toy2/dyn_auc/high_lambda/l2.pdf}
%     }
%     \caption{Dynamics of a run of \cref{alg:sec3} on \cref{example:toy2}.}\label{fig:dynamics_toy2}
% \end{figure}
% 
% \begin{figure}[h]
%     \centering
%     \subfigure{
%     \includegraphics[width=0.21\linewidth]{figures/expes/toy2/dyn_ptw/med_lambda/cost.pdf}
%     \includegraphics[width=0.21\linewidth]{figures/expes/toy2/dyn_ptw/med_lambda/auc.pdf}
%     \includegraphics[width=0.21\linewidth]{figures/expes/toy2/dyn_ptw/med_lambda/l2.pdf}
%     }
%     \subfigure[$\lambda=0.1$]{
%     \includegraphics[width=0.20\linewidth]{figures/expes/toy2/dyn_ptw/med_lambda/fprs.pdf}
%     \includegraphics[width=0.20\linewidth]{figures/expes/toy2/dyn_ptw/med_lambda/tprs.pdf}
%     \includegraphics[width=0.20\linewidth]{figures/expes/toy2/dyn_ptw/med_lambda/thres.pdf}
%     \includegraphics[width=0.20\linewidth]{figures/expes/toy2/dyn_ptw/med_lambda/cs.pdf}
%     }
%     \subfigure{
%     \includegraphics[width=0.21\linewidth]{figures/expes/toy2/dyn_ptw/high_lambda/cost.pdf}
%     \includegraphics[width=0.21\linewidth]{figures/expes/toy2/dyn_ptw/high_lambda/auc.pdf}
%     \includegraphics[width=0.21\linewidth]{figures/expes/toy2/dyn_ptw/high_lambda/l2.pdf}
%     }
%     \subfigure[$\lambda = 1$]{
%     \includegraphics[width=0.20\linewidth]{figures/expes/toy2/dyn_ptw/high_lambda/fprs.pdf}
%     \includegraphics[width=0.20\linewidth]{figures/expes/toy2/dyn_ptw/high_lambda/tprs.pdf}
%     \includegraphics[width=0.20\linewidth]{figures/expes/toy2/dyn_ptw/high_lambda/thres.pdf}
%     \includegraphics[width=0.20\linewidth]{figures/expes/toy2/dyn_ptw/high_lambda/cs.pdf}
%     }
%     \caption{Dynamics of a run of \cref{alg:sec4} on \cref{example:toy2}.}\label{fig:dynamics_toy2_ptw}
% \end{figure}
% 
% 
% \begin{figure}[h]
%     \centering
%     \subfigure{
%     \includegraphics[width=0.25\linewidth]{figures/expes/adult/auc_cons/med_lamb/dyn/cost.pdf}
%     \includegraphics[width=0.25\linewidth]{figures/expes/adult/auc_cons/med_lamb/dyn/auc.pdf}
%     \includegraphics[width=0.25\linewidth]{figures/expes/adult/auc_cons/med_lamb/dyn/f_auc.pdf}
%     }
%     \subfigure[$\lambda =0.1$]{
%     \includegraphics[width=0.25\linewidth]{figures/expes/adult/auc_cons/med_lamb/dyn/c.pdf}
%     \includegraphics[width=0.25\linewidth]{figures/expes/adult/auc_cons/med_lamb/dyn/l2.pdf}
%     }
%     \subfigure{
%     \includegraphics[width=0.25\linewidth]{figures/expes/adult/auc_cons/high_lamb/dyn/cost.pdf}
%     \includegraphics[width=0.25\linewidth]{figures/expes/adult/auc_cons/high_lamb/dyn/auc.pdf}
%     \includegraphics[width=0.25\linewidth]{figures/expes/adult/auc_cons/high_lamb/dyn/f_auc.pdf}
%     }
%     \subfigure[$\lambda = 1$]{
%     \includegraphics[width=0.25\linewidth]{figures/expes/adult/auc_cons/high_lamb/dyn/c.pdf}
%     \includegraphics[width=0.25\linewidth]{figures/expes/adult/auc_cons/high_lamb/dyn/l2.pdf}
%     }
%     \caption{Dynamics of a run of \cref{alg:sec3} on \textit{Adult}.}\label{fig:dynamics_adult}
% \end{figure}
% 
% 
% \begin{figure}[h]
%     \centering
%     \subfigure{
%     \includegraphics[width=0.25\linewidth]{figures/expes/compas/auc_cons/med_lamb/dyn/cost.pdf}
%     \includegraphics[width=0.25\linewidth]{figures/expes/compas/auc_cons/med_lamb/dyn/auc.pdf}
%     \includegraphics[width=0.25\linewidth]{figures/expes/compas/auc_cons/med_lamb/dyn/f_auc.pdf}
%     }
%     \subfigure[$\lambda =0.1$]{
%     \includegraphics[width=0.25\linewidth]{figures/expes/compas/auc_cons/med_lamb/dyn/c.pdf}
%     \includegraphics[width=0.25\linewidth]{figures/expes/compas/auc_cons/med_lamb/dyn/l2.pdf}
%     }
%     \subfigure{
%     \includegraphics[width=0.25\linewidth]{figures/expes/compas/auc_cons/high_lamb/dyn/cost.pdf}
%     \includegraphics[width=0.25\linewidth]{figures/expes/compas/auc_cons/high_lamb/dyn/auc.pdf}
%     \includegraphics[width=0.25\linewidth]{figures/expes/compas/auc_cons/high_lamb/dyn/f_auc.pdf}
%     }
%     \subfigure[$\lambda = 1$]{
%     \includegraphics[width=0.25\linewidth]{figures/expes/compas/auc_cons/high_lamb/dyn/c.pdf}
%     \includegraphics[width=0.25\linewidth]{figures/expes/compas/auc_cons/high_lamb/dyn/l2.pdf}
%     }
%     \caption{Dynamics of a run of \cref{alg:sec3} on \textit{Compas}.}\label{fig:dynamics_compas}
% \end{figure}
% 
% \begin{figure}[h]
%     \centering
%     \subfigure{
%     \includegraphics[width=0.25\linewidth]{figures/expes/bank/auc_cons/med_lamb/dyn/cost.pdf}
%     \includegraphics[width=0.25\linewidth]{figures/expes/bank/auc_cons/med_lamb/dyn/auc.pdf}
%     \includegraphics[width=0.25\linewidth]{figures/expes/bank/auc_cons/med_lamb/dyn/f_auc.pdf}
%     }
%     \subfigure[$\lambda =0.1$]{
%     \includegraphics[width=0.25\linewidth]{figures/expes/bank/auc_cons/med_lamb/dyn/c.pdf}
%     \includegraphics[width=0.25\linewidth]{figures/expes/bank/auc_cons/med_lamb/dyn/l2.pdf}
%     }
%     \subfigure{
%     \includegraphics[width=0.25\linewidth]{figures/expes/bank/auc_cons/high_lamb/dyn/cost.pdf}
%     \includegraphics[width=0.25\linewidth]{figures/expes/bank/auc_cons/high_lamb/dyn/auc.pdf}
%     \includegraphics[width=0.25\linewidth]{figures/expes/bank/auc_cons/high_lamb/dyn/f_auc.pdf}
%     }
%     \subfigure[$\lambda = 1$]{
%     \includegraphics[width=0.25\linewidth]{figures/expes/bank/auc_cons/high_lamb/dyn/c.pdf}
%     \includegraphics[width=0.25\linewidth]{figures/expes/bank/auc_cons/high_lamb/dyn/l2.pdf}
%     }
%     \caption{Dynamics of a run of \cref{alg:sec3} on \textit{Bank}.}\label{fig:dynamics_bank}
% \end{figure}
% 
% 
% 
% \begin{figure}[h]
%     \centering
% \subfigure{
% \includegraphics[width=0.21\linewidth]{figures/expes/adult/ptw_cons/med_lamb/dyn/cost.pdf}
% \includegraphics[width=0.21\linewidth]{figures/expes/adult/ptw_cons/med_lamb/dyn/auc.pdf}
% \includegraphics[width=0.21\linewidth]{figures/expes/adult/ptw_cons/med_lamb/dyn/l2.pdf}
% }
% \subfigure[$\lambda=0.1$]{
% \includegraphics[width=0.20\linewidth]{figures/expes/adult/ptw_cons/med_lamb/dyn/fprs.pdf}
% \includegraphics[width=0.20\linewidth]{figures/expes/adult/ptw_cons/med_lamb/dyn/tprs.pdf}
% \includegraphics[width=0.20\linewidth]{figures/expes/adult/ptw_cons/med_lamb/dyn/thres.pdf}
% \includegraphics[width=0.20\linewidth]{figures/expes/adult/ptw_cons/med_lamb/dyn/cs.pdf}
% }
% \subfigure{
% \includegraphics[width=0.21\linewidth]{figures/expes/adult/ptw_cons/high_lamb/dyn/cost.pdf}
% \includegraphics[width=0.21\linewidth]{figures/expes/adult/ptw_cons/high_lamb/dyn/auc.pdf}
% \includegraphics[width=0.21\linewidth]{figures/expes/adult/ptw_cons/high_lamb/dyn/l2.pdf}
% }
% \subfigure[$\lambda= 1$]{
% \includegraphics[width=0.20\linewidth]{figures/expes/adult/ptw_cons/high_lamb/dyn/fprs.pdf}
% \includegraphics[width=0.20\linewidth]{figures/expes/adult/ptw_cons/high_lamb/dyn/tprs.pdf}
% \includegraphics[width=0.20\linewidth]{figures/expes/adult/ptw_cons/high_lamb/dyn/thres.pdf}
% \includegraphics[width=0.20\linewidth]{figures/expes/adult/ptw_cons/high_lamb/dyn/cs.pdf}
% }
%     \caption{Dynamics of a run of \cref{alg:sec4} on \textit{Adult}.}\label{fig:dynamics_adult_ptw}
% \end{figure}
% 
% \begin{figure}[h]
%     \centering
% \subfigure{
% \includegraphics[width=0.21\linewidth]{figures/expes/compas/ptw_cons/med_lamb/dyn/cost.pdf}
% \includegraphics[width=0.21\linewidth]{figures/expes/compas/ptw_cons/med_lamb/dyn/auc.pdf}
% \includegraphics[width=0.21\linewidth]{figures/expes/compas/ptw_cons/med_lamb/dyn/l2.pdf}
% }
% \subfigure[$\lambda=0.1$]{
% \includegraphics[width=0.20\linewidth]{figures/expes/compas/ptw_cons/med_lamb/dyn/fprs.pdf}
% \includegraphics[width=0.20\linewidth]{figures/expes/compas/ptw_cons/med_lamb/dyn/tprs.pdf}
% \includegraphics[width=0.20\linewidth]{figures/expes/compas/ptw_cons/med_lamb/dyn/thres.pdf}
% \includegraphics[width=0.20\linewidth]{figures/expes/compas/ptw_cons/med_lamb/dyn/cs.pdf}
% }
% \subfigure{
% \includegraphics[width=0.21\linewidth]{figures/expes/compas/ptw_cons/high_lamb/dyn/cost.pdf}
% \includegraphics[width=0.21\linewidth]{figures/expes/compas/ptw_cons/high_lamb/dyn/auc.pdf}
% \includegraphics[width=0.21\linewidth]{figures/expes/compas/ptw_cons/high_lamb/dyn/l2.pdf}
% }
% \subfigure[$\lambda= 1$]{
% \includegraphics[width=0.20\linewidth]{figures/expes/compas/ptw_cons/high_lamb/dyn/fprs.pdf}
% \includegraphics[width=0.20\linewidth]{figures/expes/compas/ptw_cons/high_lamb/dyn/tprs.pdf}
% \includegraphics[width=0.20\linewidth]{figures/expes/compas/ptw_cons/high_lamb/dyn/thres.pdf}
% \includegraphics[width=0.20\linewidth]{figures/expes/compas/ptw_cons/high_lamb/dyn/cs.pdf}
% }
%     \caption{Dynamics of a run of \cref{alg:sec4} on \textit{Compas}.}\label{fig:dynamics_compas_ptw}
% \end{figure}
% 
% 
% \begin{figure}[h]
%     \centering
% \subfigure{
% \includegraphics[width=0.21\linewidth]{figures/expes/bank/ptw_cons/med_lamb/dyn/cost.pdf}
% \includegraphics[width=0.21\linewidth]{figures/expes/bank/ptw_cons/med_lamb/dyn/auc.pdf}
% \includegraphics[width=0.21\linewidth]{figures/expes/bank/ptw_cons/med_lamb/dyn/l2.pdf}
% }
% \subfigure[$\lambda=0.1$]{
% \includegraphics[width=0.20\linewidth]{figures/expes/bank/ptw_cons/med_lamb/dyn/fprs.pdf}
% \includegraphics[width=0.20\linewidth]{figures/expes/bank/ptw_cons/med_lamb/dyn/tprs.pdf}
% \includegraphics[width=0.20\linewidth]{figures/expes/bank/ptw_cons/med_lamb/dyn/thres.pdf}
% \includegraphics[width=0.20\linewidth]{figures/expes/bank/ptw_cons/med_lamb/dyn/cs.pdf}
% }
% \subfigure{
% \includegraphics[width=0.21\linewidth]{figures/expes/bank/ptw_cons/high_lamb/dyn/cost.pdf}
% \includegraphics[width=0.21\linewidth]{figures/expes/bank/ptw_cons/high_lamb/dyn/auc.pdf}
% \includegraphics[width=0.21\linewidth]{figures/expes/bank/ptw_cons/high_lamb/dyn/l2.pdf}
% }
% \subfigure[$\lambda= 1$]{
% \includegraphics[width=0.20\linewidth]{figures/expes/bank/ptw_cons/high_lamb/dyn/fprs.pdf}
% \includegraphics[width=0.20\linewidth]{figures/expes/bank/ptw_cons/high_lamb/dyn/tprs.pdf}
% \includegraphics[width=0.20\linewidth]{figures/expes/bank/ptw_cons/high_lamb/dyn/thres.pdf}
% \includegraphics[width=0.20\linewidth]{figures/expes/bank/ptw_cons/high_lamb/dyn/cs.pdf}
% }
%     \caption{Dynamics of a run of \cref{alg:sec4} on \textit{Bank}.}\label{fig:dynamics_bank_ptw}
% \end{figure}
% 
% 
% \subsection{ROC curves}
% 
% \robin{list of figures}
% 
% \begin{figure}[h]
% \centering
% \begin{minipage}{.45\textwidth}
% \centering
%     \includegraphics[width=0.95\columnwidth]{figures/expes/toy1/avg_rocs/high_lambda/legend-sec3.pdf}
%     \subfigure[$\lambda = 0.1$]{\label{fig:ex-square-sol-low-lambda}
%     \includegraphics[width=0.47\columnwidth]{figures/expes/toy1/avg_rocs/med_lambda/roc_curves_quant_sec3.pdf}}
%     \subfigure[$\lambda = 1$]{\label{fig:ex-square-sol-high-lambda}
%     \includegraphics[width=0.47\columnwidth]{figures/expes/toy1/avg_rocs/high_lambda/roc_curves_quant_sec3.pdf}
%     }
% \end{minipage}
% \begin{minipage}{.45\textwidth}
% \centering
%     \includegraphics[width=0.95\columnwidth]{figures/expes/toy1/avg_rocs/high_lambda/legend-sec4.pdf}
%     \subfigure[$\lambda = 0.1$]{\label{fig:ex-square-sol-low-lambda}
%     \includegraphics[width=0.47\columnwidth]{figures/expes/toy1/avg_rocs/med_lambda/roc_curves_quant_sec4.pdf}}
%     \subfigure[$\lambda = 1$]{\label{fig:ex-square-sol-high-lambda}
%     \includegraphics[width=0.47\columnwidth]{figures/expes/toy1/avg_rocs/high_lambda/roc_curves_quant_sec4.pdf}
%     }
% \end{minipage}
% \caption{Result of \cref{example-square} with \cref{alg:sec3}.}\label{fig:avg_roc_toy1_alg1}
% 
% \bigskip
% \bigskip
%     \begin{minipage}{.45\textwidth}
%     \centering
%     \subfigure[$\lambda = 0.1$]{\label{fig:ex-square-sol-low-lambda}
%     \includegraphics[width=0.47\columnwidth]{figures/expes/toy2/avg_rocs/auc_cons/med_lambda/roc_curves_quant_sec3.pdf}}
%     \subfigure[$\lambda = 1$]{\label{fig:ex-square-sol-high-lambda}
% 	\includegraphics[width=0.47\columnwidth]{figures/expes/toy2/avg_rocs/auc_cons/high_lambda/roc_curves_quant_sec3.pdf}
%     }
%     \end{minipage}
%     \begin{minipage}{.45\textwidth}
%     \centering
%     \subfigure[$\lambda = 0.1$]{\label{fig:ex-square-sol-low-lambda}
%     \includegraphics[width=0.47\columnwidth]{figures/expes/toy2/avg_rocs/auc_cons/med_lambda/roc_curves_quant_sec4.pdf}}
%     \subfigure[$\lambda = 1$]{\label{fig:ex-square-sol-high-lambda}
% 	\includegraphics[width=0.47\columnwidth]{figures/expes/toy2/avg_rocs/auc_cons/high_lambda/roc_curves_quant_sec4.pdf}
%     }
%     \end{minipage}
%     \caption{result of \cref{example:toy2} with \cref{alg:sec3}.}\label{fig:avg_roc_toy2_alg1}
% 
% \bigskip
% \bigskip
%     \begin{minipage}{.45\textwidth}
%     \centering
%     \subfigure[$\lambda = 0.1$]{\label{fig:ex-square-sol-low-lambda}
%     \includegraphics[width=0.47\columnwidth]{figures/expes/toy2/avg_rocs/ptw_cons/med_lambda/roc_curves_quant_sec3.pdf}}
%     \subfigure[$\lambda = 1$]{\label{fig:ex-square-sol-high-lambda}
% 	\includegraphics[width=0.47\columnwidth]{figures/expes/toy2/avg_rocs/ptw_cons/high_lambda/roc_curves_quant_sec3.pdf}
%     }
%     \end{minipage}
%     \begin{minipage}{.45\textwidth}
%     \centering
%     \subfigure[$\lambda = 0.1$]{\label{fig:ex-square-sol-low-lambda}
%     \includegraphics[width=0.47\columnwidth]{figures/expes/toy2/avg_rocs/ptw_cons/med_lambda/roc_curves_quant_sec4.pdf}}
%     \subfigure[$\lambda = 1$]{\label{fig:ex-square-sol-high-lambda}
% 	\includegraphics[width=0.47\columnwidth]{figures/expes/toy2/avg_rocs/ptw_cons/high_lambda/roc_curves_quant_sec4.pdf}
%     }
%     \end{minipage}
%     \caption{Result of \cref{example:toy2} with \cref{alg:sec4}.\label{fig:avg_roc_toy2_alg2}
%     }
% 
%     \centering
% \caption{based on 100 independent runs of the proposed algorithms with different generated
%     datasets, we have computed the 100 resulting roc curves on each
%     a different, new generated dataset.
%     This is meant to show that the learning procedure recovers the expected solution
%     with little variance when data is abundant.
%     We show the pointwise median and 95\% confidence intervals (CI) 
%     of the 100 ROC curves for \cref{alg:sec3} for \cref{example-square}
%     and both algorithms for \cref{example:toy2}, for two example $\lambda$ parameters.
%     The two left-hand side figures show the $\roc_{H^{(0)}_s, G^{(0)}_s}$ and
%     $\roc_{H^{(1)}_s, G^{(1)}_s}$, while the two right-hand side figures show the
%     $\roc_{H^{(0)}_s, H^{(1)}_s}$ and $\roc_{G^{(0)}_s, G^{(1)}_s}$,
%     as explicited by the legend above.
%     }\label{fig:avg_roc}
% \end{figure}
% 
% 
% 
% \begin{figure}[h]
% \centering
% \begin{minipage}{.45\textwidth}
% \centering
%     \includegraphics[width=0.95\columnwidth]{figures/expes/leg_sec3.pdf}
%     \subfigure[$\lambda = 0.1$]{\label{fig:}
%     \includegraphics[width=0.47\columnwidth]{figures/expes/german/auc_cons/med_lamb/roc_sec3.pdf}}
%     \subfigure[$\lambda = 1$]{\label{fig:}
%     \includegraphics[width=0.47\columnwidth]{figures/expes/german/auc_cons/high_lamb/roc_sec3.pdf}
%     }
% \end{minipage}
% \begin{minipage}{.45\textwidth}
% \centering
%     \includegraphics[width=0.95\columnwidth]{figures/expes/leg_sec4.pdf}
%     \subfigure[$\lambda = 0.1$]{\label{fig:}
%     \includegraphics[width=0.47\columnwidth]{figures/expes/german/auc_cons/med_lamb/roc_sec4.pdf}}
%     \subfigure[$\lambda = 1$]{\label{fig:}
%     \includegraphics[width=0.47\columnwidth]{figures/expes/german/auc_cons/high_lamb/roc_sec4.pdf}
%     }
% \end{minipage}
% \caption{Result of \textit{German} with \cref{alg:sec3}.}\label{fig:res-german-alg1}
% 
% \begin{minipage}{.45\textwidth}
% \centering
%     \subfigure[$\lambda = 0.1$]{\label{fig:}
%     \includegraphics[width=0.47\columnwidth]{figures/expes/adult/auc_cons/med_lamb/roc_sec3.pdf}}
%     \subfigure[$\lambda = 1$]{\label{fig:}
%     \includegraphics[width=0.47\columnwidth]{figures/expes/adult/auc_cons/high_lamb/roc_sec3.pdf}
%     }
% \end{minipage}
% \begin{minipage}{.45\textwidth}
% \centering
%     \subfigure[$\lambda = 0.1$]{\label{fig:}
%     \includegraphics[width=0.47\columnwidth]{figures/expes/adult/auc_cons/med_lamb/roc_sec4.pdf}}
%     \subfigure[$\lambda = 1$]{\label{fig:}
%     \includegraphics[width=0.47\columnwidth]{figures/expes/adult/auc_cons/high_lamb/roc_sec4.pdf}
%     }
% \end{minipage}
% \caption{Result of \textit{Adult} with \cref{alg:sec3}.}\label{fig:res-adult-alg1}
% 
% \begin{minipage}{.45\textwidth}
% \centering
%     \subfigure[$\lambda = 0.1$]{\label{fig:}
%     \includegraphics[width=0.47\columnwidth]{figures/expes/compas/auc_cons/med_lamb/roc_sec3.pdf}}
%     \subfigure[$\lambda = 1$]{\label{fig:}
%     \includegraphics[width=0.47\columnwidth]{figures/expes/compas/auc_cons/high_lamb/roc_sec3.pdf}
%     }
% \end{minipage}
% \begin{minipage}{.45\textwidth}
% \centering
%     \subfigure[$\lambda = 0.1$]{\label{fig:}
%     \includegraphics[width=0.47\columnwidth]{figures/expes/compas/auc_cons/med_lamb/roc_sec4.pdf}}
%     \subfigure[$\lambda = 1$]{\label{fig:}
%     \includegraphics[width=0.47\columnwidth]{figures/expes/compas/auc_cons/high_lamb/roc_sec4.pdf}
%     }
% \end{minipage}
% \caption{Result of \textit{Compas} with \cref{alg:sec3}.}\label{fig:res-compas-alg1}
% 
% \centering
% \begin{minipage}{.45\textwidth}
% \centering
%     \subfigure[$\lambda = 0.1$]{\label{fig:}
%     \includegraphics[width=0.47\columnwidth]{figures/expes/bank/auc_cons/med_lamb/roc_sec3.pdf}}
%     \subfigure[$\lambda = 1$]{\label{fig:}
%     \includegraphics[width=0.47\columnwidth]{figures/expes/bank/auc_cons/high_lamb/roc_sec3.pdf}
%     }
% \end{minipage}
% \begin{minipage}{.45\textwidth}
% \centering
%     \subfigure[$\lambda = 0.1$]{\label{fig:}
%     \includegraphics[width=0.47\columnwidth]{figures/expes/bank/auc_cons/med_lamb/roc_sec4.pdf}}
%     \subfigure[$\lambda = 1$]{\label{fig:}
%     \includegraphics[width=0.47\columnwidth]{figures/expes/bank/auc_cons/high_lamb/roc_sec4.pdf}
%     }
% \end{minipage}
% \caption{Result of \textit{Bank} with \cref{alg:sec3}.}\label{fig:res-bank-alg1}
% 
%     \centering
%     \caption{Results of \cref{alg:sec3} on the real data.}\label{fig:results-real-data-fig1}
% \end{figure}
% 
% 
% \begin{figure}[h]
% \centering
% \begin{minipage}{.45\textwidth}
% \centering
%     \includegraphics[width=0.95\columnwidth]{figures/expes/leg_sec3.pdf}
%     \subfigure[$\lambda = 0.1$]{\label{fig:}
%     \includegraphics[width=0.47\columnwidth]{figures/expes/adult/ptw_cons/med_lamb/roc_sec3.pdf}}
%     \subfigure[$\lambda = 1$]{\label{fig:}
%     \includegraphics[width=0.47\columnwidth]{figures/expes/adult/ptw_cons/high_lamb/roc_sec3.pdf}
%     }
% \end{minipage}
% \begin{minipage}{.45\textwidth}
% \centering
%     \includegraphics[width=0.95\columnwidth]{figures/expes/leg_sec4.pdf}
%     \subfigure[$\lambda = 0.1$]{\label{fig:}
%     \includegraphics[width=0.47\columnwidth]{figures/expes/adult/ptw_cons/med_lamb/roc_sec4.pdf}}
%     \subfigure[$\lambda = 1$]{\label{fig:}
%     \includegraphics[width=0.47\columnwidth]{figures/expes/adult/ptw_cons/high_lamb/roc_sec4.pdf}
%     }
% \end{minipage}
% \caption{Result of \textit{Adult} with \cref{alg:sec4}.}\label{fig:res-adult-alg2}
% 
% \bigskip
% \begin{minipage}{.45\textwidth}
% \centering
%     \subfigure[$\lambda = 0.1$]{\label{fig:}
%     \includegraphics[width=0.47\columnwidth]{figures/expes/compas/ptw_cons/med_lamb/roc_sec3.pdf}}
%     \subfigure[$\lambda = 1$]{\label{fig:}
%     \includegraphics[width=0.47\columnwidth]{figures/expes/compas/ptw_cons/high_lamb/roc_sec3.pdf}
%     }
% \end{minipage}
% \begin{minipage}{.45\textwidth}
% \centering
%     \subfigure[$\lambda = 0.1$]{\label{fig:}
%     \includegraphics[width=0.47\columnwidth]{figures/expes/compas/ptw_cons/med_lamb/roc_sec4.pdf}}
%     \subfigure[$\lambda = 1$]{\label{fig:}
%     \includegraphics[width=0.47\columnwidth]{figures/expes/compas/ptw_cons/high_lamb/roc_sec4.pdf}
%     }
% \end{minipage}
% \caption{Result of \textit{Compas} with \cref{alg:sec4}.}\label{fig:res-compas-alg2}
% 
% \bigskip
% \bigskip
% \begin{minipage}{.45\textwidth}
% \centering
%     \subfigure[$\lambda = 0.1$]{\label{fig:}
%     \includegraphics[width=0.47\columnwidth]{figures/expes/bank/ptw_cons/med_lamb/roc_sec3.pdf}}
%     \subfigure[$\lambda = 1$]{\label{fig:}
%     \includegraphics[width=0.47\columnwidth]{figures/expes/bank/ptw_cons/high_lamb/roc_sec3.pdf}
%     }
% \end{minipage}
% \begin{minipage}{.45\textwidth}
% \centering
%     \subfigure[$\lambda = 0.1$]{\label{fig:}
%     \includegraphics[width=0.47\columnwidth]{figures/expes/bank/ptw_cons/med_lamb/roc_sec4.pdf}}
%     \subfigure[$\lambda = 1$]{\label{fig:}
%     \includegraphics[width=0.47\columnwidth]{figures/expes/bank/ptw_cons/high_lamb/roc_sec4.pdf}
%     }
% \end{minipage}
% \caption{Result of \textit{Bank} with \cref{alg:sec4}.}\label{fig:fig:res-bank-alg2}
% 
%     \centering
%     \caption{Results of \cref{alg:sec4} on the real data.
%     }\label{fig:results-real-data-fig3}
% \end{figure}

% \begin{figure}[h]
% \centering
% \begin{minipage}{.45\textwidth}
% \centering
%     \includegraphics[width=0.95\columnwidth]{figures/expes/}
%     \subfigure[$\lambda = 0.1$]{\label{fig:}
%     \includegraphics[width=0.47\columnwidth]{figures/expes/}}
%     \subfigure[$\lambda = 1$]{\label{fig:}
%     \includegraphics[width=0.47\columnwidth]{figures/expes/}
%     }
% \end{minipage}
% \begin{minipage}{.45\textwidth}
% \centering
%     \includegraphics[width=0.95\columnwidth]{figures/expes/}
%     \subfigure[$\lambda = 0.1$]{\label{fig:}
%     \includegraphics[width=0.47\columnwidth]{figures/expes/}}
%     \subfigure[$\lambda = 1$]{\label{fig:}
%     \includegraphics[width=0.47\columnwidth]{figures/expes/}
%     }
% \end{minipage}
% \caption{Result of \robin{TODO} with \cref{alg:sec3}.}\label{fig:}
% 
% \bigskip
% \bigskip
%     \begin{minipage}{.45\textwidth}
%     \centering
%     \subfigure[$\lambda = 0.1$]{\label{fig:}
%     \includegraphics[width=0.47\columnwidth]{figures/expes/}}
%     \subfigure[$\lambda = 1$]{\label{fig:}
% 	\includegraphics[width=0.47\columnwidth]{figures/expes/}
%     }
%     \end{minipage}
%     \begin{minipage}{.45\textwidth}
%     \centering
%     \subfigure[$\lambda = 0.1$]{\label{fig:}
%     \includegraphics[width=0.47\columnwidth]{figures/expes/}}
%     \subfigure[$\lambda = 1$]{\label{fig:}
% 	\includegraphics[width=0.47\columnwidth]{figures/expes/}
%     }
%     \end{minipage}
%     \caption{result of \robin{TODO} with \cref{alg:sec3}.}\label{fig:}
% \bigskip
% \bigskip
%     \begin{minipage}{.45\textwidth}
%     \centering
%     \subfigure[$\lambda = 0.1$]{\label{fig:}
%     \includegraphics[width=0.47\columnwidth]{figures/expes/}}
%     \subfigure[$\lambda = 1$]{\label{fig:}
% 	\includegraphics[width=0.47\columnwidth]{figures/expes/}
%     }
%     \end{minipage}
%     \begin{minipage}{.45\textwidth}
%     \centering
%     \subfigure[$\lambda = 0.1$]{\label{fig:}
%     \includegraphics[width=0.47\columnwidth]{figures/expes/}}
%     \subfigure[$\lambda = 1$]{\label{fig:}
% 	\includegraphics[width=0.47\columnwidth]{figures/expes/}
%     }
%     \end{minipage}
%     \caption{Result of \robin{TODO} with \cref{alg:sec3}.\label{fig:}
%     }
% 
%     \centering
% \caption{TODO}\label{fig:fig-results-real-data-fig2}
% \end{figure}
